# Supplementary material for: First-Principles Simulations of Tip Enhanced Raman Scattering Reveal Active Role of Substrate on High-Resolution Images
Source: arXiv:2211.09475 source file (2023-03-09)

a)

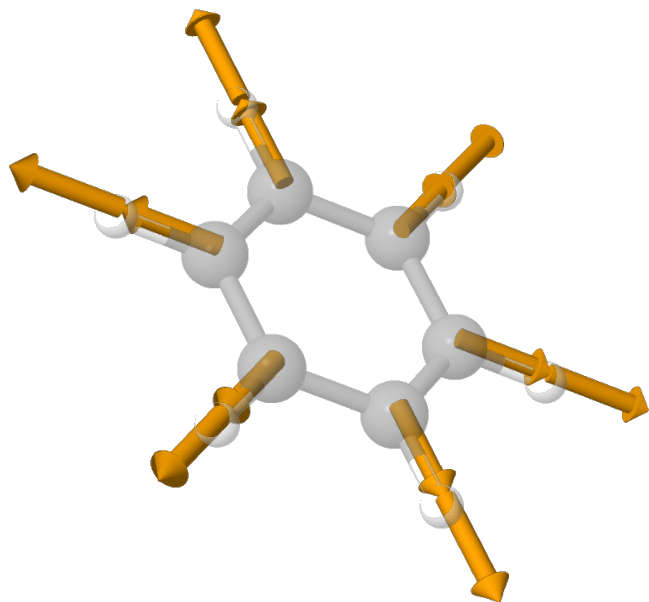

b)

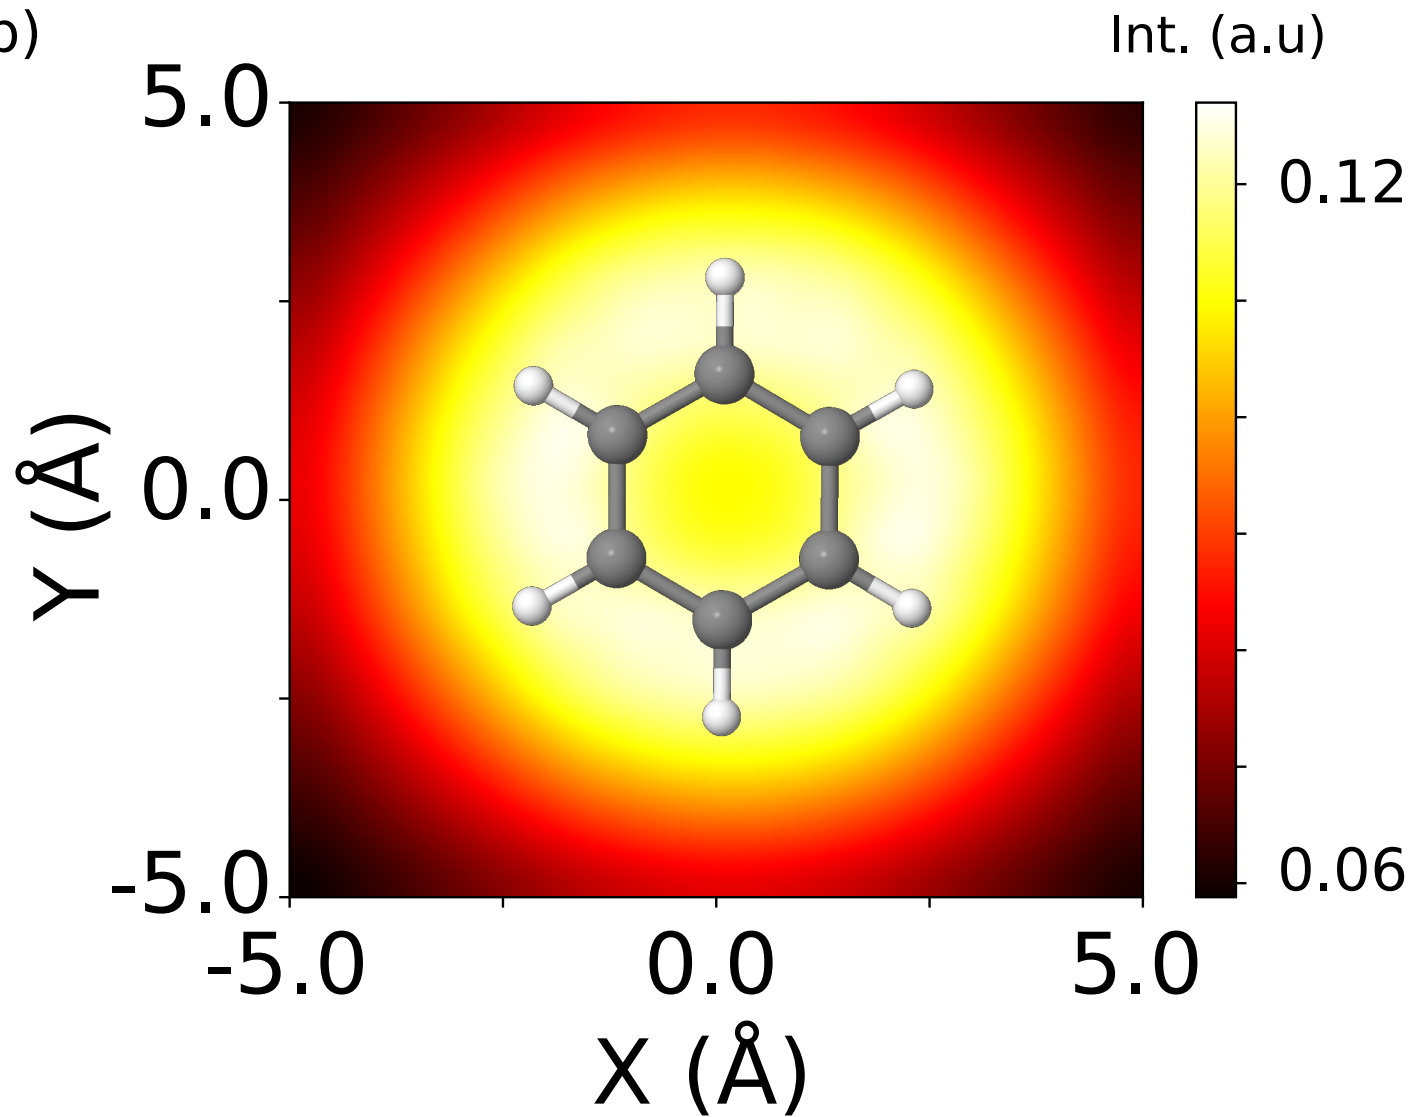

Supplement: Supplementary file 1 [file Bz_1015.pdf]
