# Supplementary material for: First-Principles Simulations of Tip Enhanced Raman Scattering Reveal Active Role of Substrate on High-Resolution Images
Source: arXiv:2211.09475 source file (2023-03-09)

a)

TD-DFT

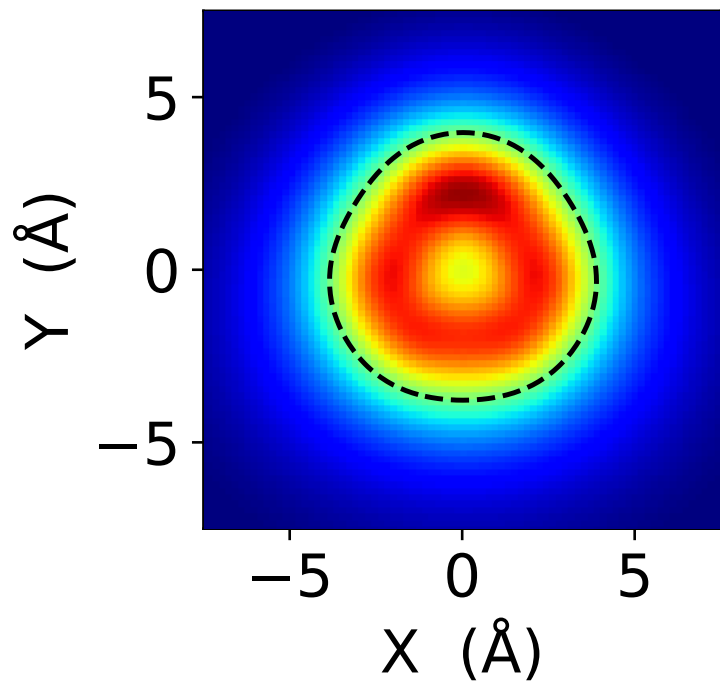

Gaussian Fit

$$\sigma_x = 3.22 \text{ Å}, \sigma_y = 3.22 \text{ Å}$$

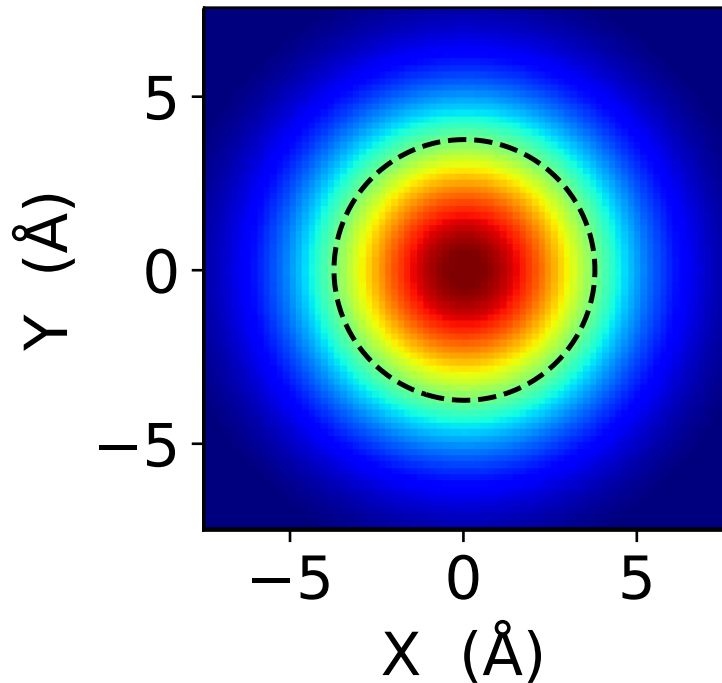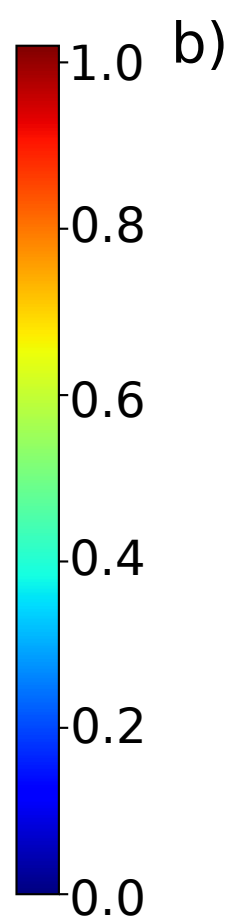

b)

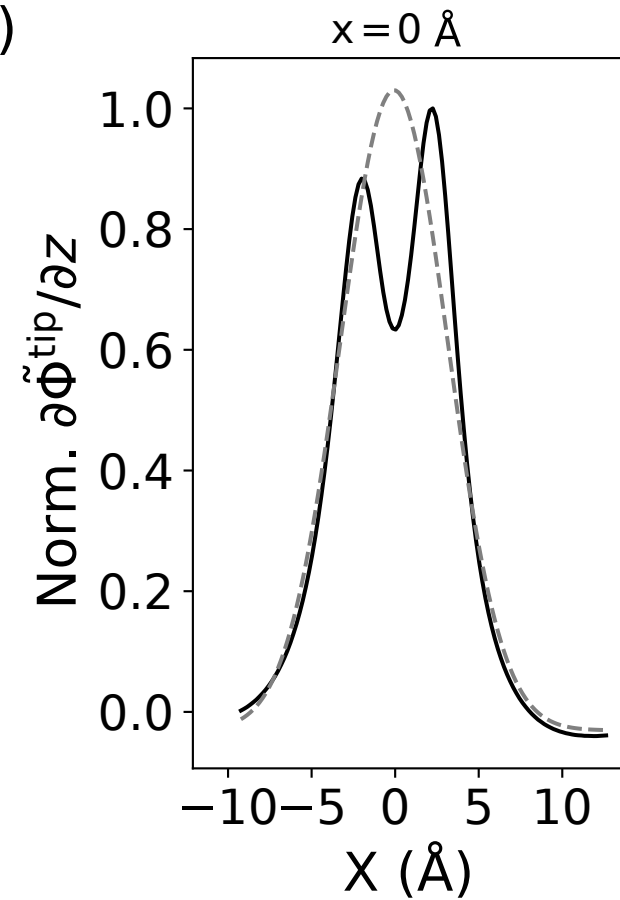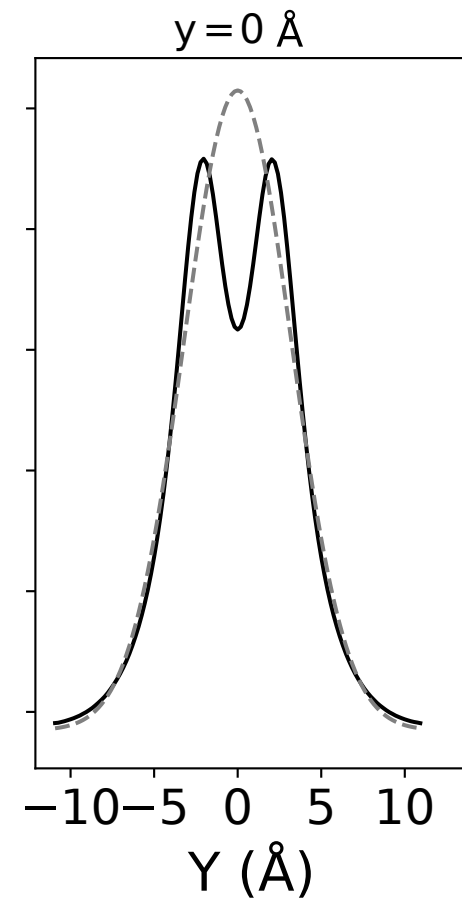

Supplement: Supplementary file 3 [file Gaussian_FitsAtipB.pdf]
