# Supplementary material for: First-Principles Simulations of Tip Enhanced Raman Scattering Reveal Active Role of Substrate on High-Resolution Images
Source: arXiv:2211.09475 source file (2023-03-09)

a)

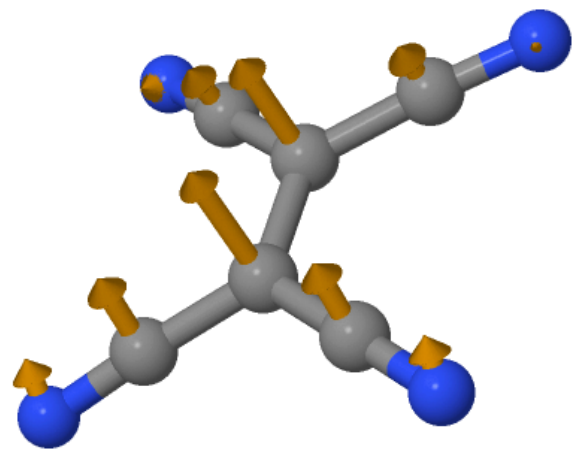

b)

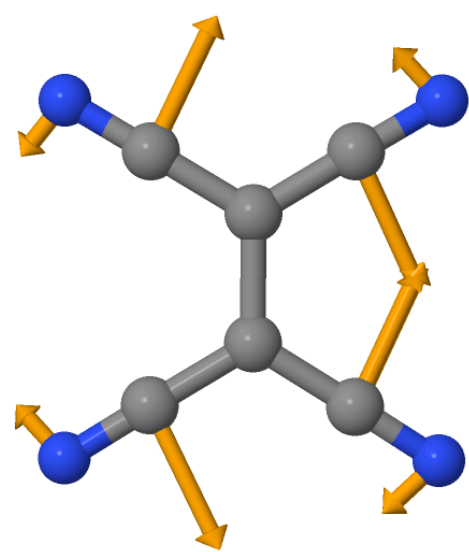

c)

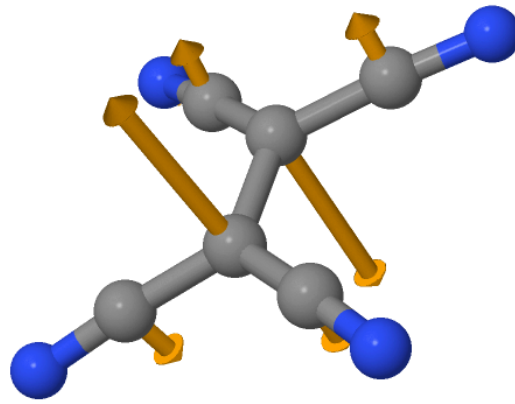

d)

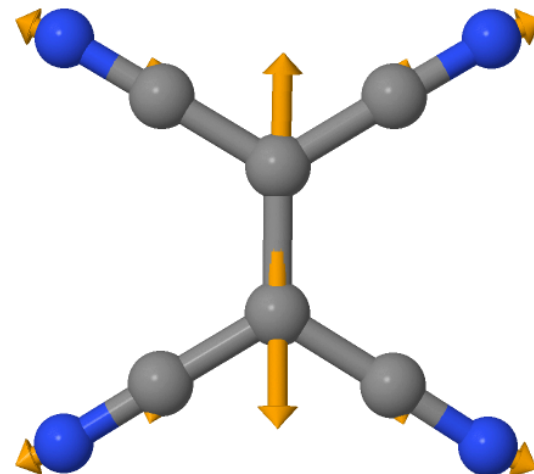

e)

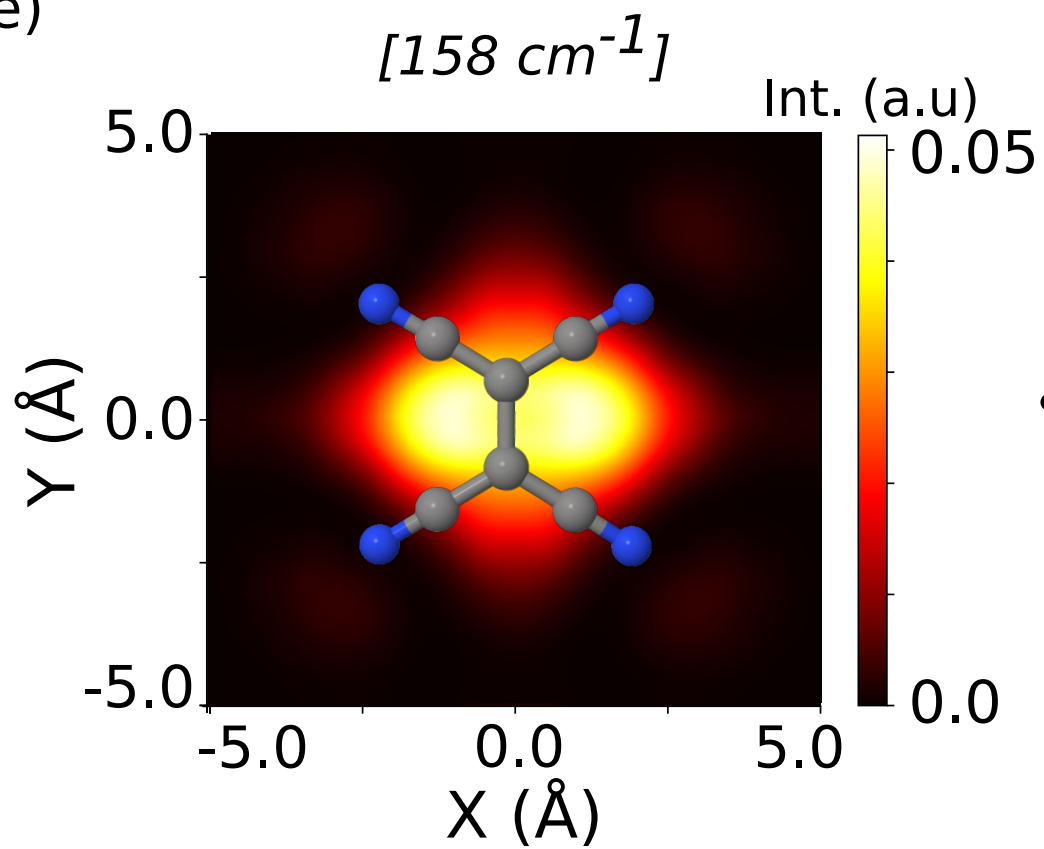

f)

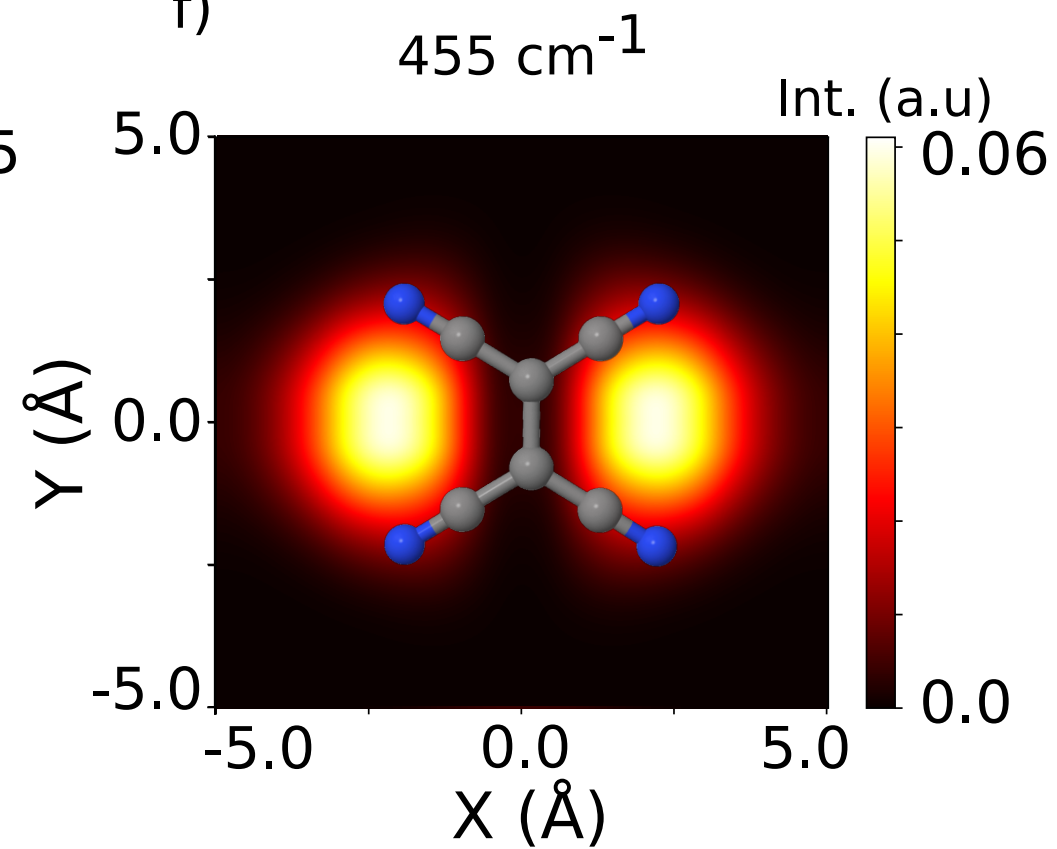

g)

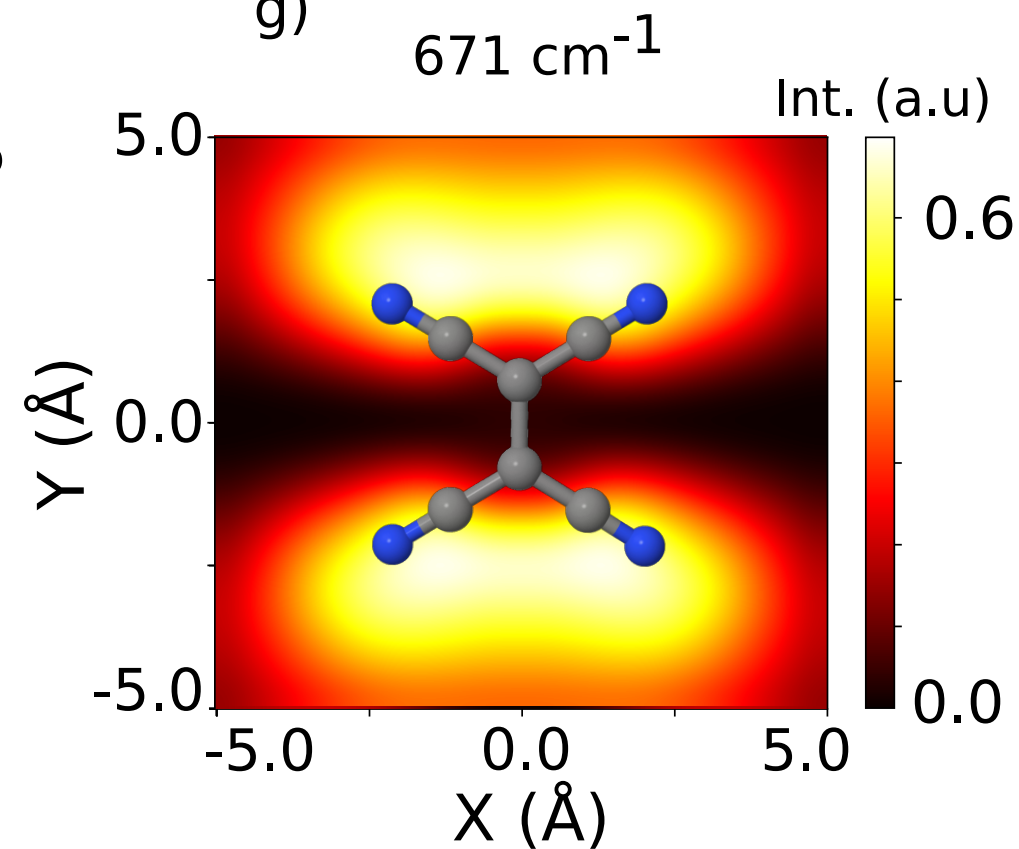

h)

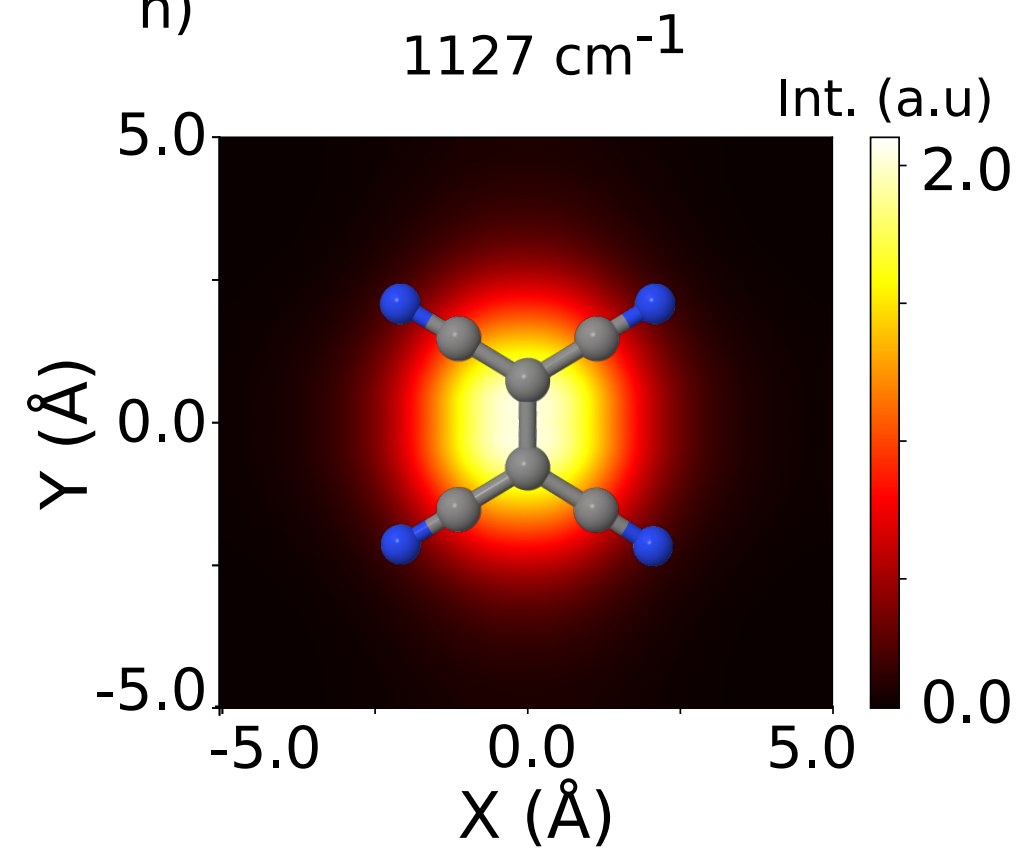

Supplement: Supplementary file 7 [file TCNE1e.pdf]
